# Supplementary material for: Z1: Efficient Test-time Scaling with Code
Source: arXiv:2504.00810 source file (2025-04-01)
Supplement: Supplementary file 1 [file appendix-qwen-base.tex]

\section{Fine-tuning Qwen2.5-Coder-7B-Base}

\subsection{Implementation Details}
To validate the effectiveness of code-related trajectory data, we fine-tune Qwen-2.5-Coder-Base (1.5B and 7B) \cite{hui2024qwen25coder} for two stages with two trajectory datasets, yielding Z1-Coder-1.5B and Z1-Coder-7B respectively.
We use a learning rate of 2e-5 for the first stage and 5e-5 for the second stage.
We train all the models with Fully Shard Data Parallel (FSDP) and set a global batch size to 1024 for 3 epochs using 2 NVIDIA A800-80G GPUs. We used greedy decoding for all results, with the maximum sequence length set to 1280.

\subsection{Evaluation Setup}
\paragraph{Datasets}
We evaluate models on HumanEval Plus and MBPP Plus \cite{liu2024your}, HumanEval pro and MBPP pro \cite{yu2024humaneval},  LiveCodeBench\cite{jain2024livecodebench} and BigCodeBench \cite{zhuo2024bigcodebench}. 
HumanEval Plus and MBPP Plus have the same problems with original HumanEval\cite{chen2021evaluating} and MBPP \cite{austin2021program} but ensure a more rigorous evaluation by providing more test cases for each problems. HumanEval Pro and MBPP Pro score LLMs on self-invoking code generation problems where LLMs are required to solve complex problems ranging in complexity from weak to strong, thereby showcasing the reasoning ability of LLMs in code generation.
LiveCodeBench benchmarks LLMs on competition-level programming task. BigCodeBench mainly focuses on more challenging and practical code generation. Through these benchmarks, we evaluate the reasoning ability of LLMs in code generations from difference perspectives.

\paragraph{Baselines}
We select these top-tier models across different size according to LiveCodeBench and BigCodeBench Leaderboard as our baseline models, including proprietary models like O1-mini \cite{o1}, GPT-4o \cite{gpt4o} and Claude-3.5-sonnet \cite{TheC3}, open-source models like Deepseek-V3 
\cite{liu2024deepseek}, DeepseekCoder-V2-Ins \cite{zhu2024deepseek2}, DeepseekCoder-Ins (6.7B and 33B) \cite{deepseek-coder}, LLaMa3.3-70B-Ins, LLaMa-3.1-70B-Ins, Qwen2.5-72B \cite{yang2024qwen2} Qwen2.5-Coder-Ins (1.5B, 7B, 33B) \cite{hui2024qwen25coder} and Yi-Coder-9B-Chat \cite{yicoder}. We use the reported results from these leaderboard whenever available.
Table \ref{tab:main-res} presents the results of Z1-Coder on all benchmarks, highlighting the following salient observations:
Using trajectory-base fine-tuning and 130K trajectory data, Z1-Coder outperforms other SoTA LLMs with comparable parameter sizes.

\begin{table}[h]
\caption{Pass@1(\%) results of different LLMs on all benchmarks. The best results in
each section are in blue , the second-best results are underlined.}
\label{tab:main-res}
\setlength{\tabcolsep}{4pt}
\resizebox{\linewidth}{!}{%

\begin{tabular}{l|cccc|cccc|cccc}
\toprule
\textbf{Model Name} & \multicolumn{2}{c}{\textbf{HumanEval}} & \multicolumn{2}{c|}{\textbf{MBPP}} & \multicolumn{4}{c}{\textbf{LiveCodeBench}} & \multicolumn{2}{|c}{\textbf{BigCodeBench}} \\
 & \textit{plus} & \textit{pro} & \textit{plus} & \textit{pro} & \textit{overall} & \textit{easy} & \textit{medium} & \textit{hard} & \textit{full set} & \textit{hard set} \\
\midrule
\multicolumn{11}{c}{\textit{Proprietary Models}} \\
\midrule
O1-mini & 90.2 & 76.2 & 78.3 & 68.3 & 58.0 & 92.3 & 83.8 & 20.4 & - & 27.0 \\
GPT-4o & 86.0 & 75.0 & 72.5 & 70.9 & 35.1 & 91.2 & 41.6 & 0.4 & - & 36.5 \\
Claude-3.5-sonnet & 86.0 & 72.6  & 74.6 & 66.4 & 31.6 & 97.7 & 27.0 & 0.0 & - & 35.1 \\
\midrule
\multicolumn{11}{c}{\textit{> 10B Models}} \\
\midrule
Deepseek-V3 & 86.6 & - & 73.0 & - & 35.1 & 92.3 & 38.6 & 2.0 & 56.1 & 39.9 \\
DeepseekCoder-V2-Ins & 84.8 & 77.4 & 76.2 & 71.4 & 27.4 & 79.2 & 27.3 & 0.0 & 54.0 & 33.1 \\
Mixtral-8x22B-Ins & 72.0 & - & 64.3 & - & 20.1 & 60.4 & 18.4 & 0.0 & 45.4 & 20.9 \\
\midrule
Qwen2.5-72B-Ins & - & 68.9 & - & 68.8 & 30.4 & 81.2 & 34.9 & 0.0 & 50.8 & 29.1 \\
% Qwen2-72B-Ins & & & & & 20.3 & 59.2 & 19.5 & 0.2 & 46.3 & 26.4 \\
LLaMA3.3-70B-Ins & - & 67.1 & - & 64.6 & 24.1 & 78.8 & 17.6 & 0.0 & 52.2 & 28.4 \\
LLaMA3.1-70B-Ins & - & 60.4 & - & 63.8 & 19.3 & 53.1 & 21.1 & 0.0 & 50.5 & 27.7 \\
\midrule
Qwen2.5Coder-32B-Ins & 87.2 & 70.1 & 75.1 & 69.8 & 30.1 & 81.2 & 34.1 & 0.0 & 53.5 & 33.8 \\
DeepseekCoder-33B-Ins & 75.0 & 56.7 & 70.1 & 64.0 & 21.5 & 65.4 & 19.2 & 0.0 & 46.5 & 20.9 \\
\midrule
\multicolumn{11}{c}{\textit{< 10B Models}} \\
\midrule
Qwen2.5-Coder-1.5B-Ins      &  66.5          &  33.5         &  59.4          &  42.1         &  8.7  & 24.6 & 8.9 &  0.0  & 32.7 & 6.1 \\
\rowcolor{lightblue}
Z1-Coder-1.5B & 72.0 & 51.2 & 61.9 & 53.2 & 11.3 & 37.3 & 8.1 &  0.0 & 39.6 & 14.9 \\
\midrule
DeepseekCoder-6.7B-Ins & 71.3 & 55.5 & 65.6 & 57.1 & 16.1 & 49.6 & 13.8 & 0.0 & 43.8 & 15.5 \\
Yi-Coder-9B-Chat & 74.4 & 59.8 & 69.3 & \underline{64.8} & \underline{19.3} & 59.2 & \underline{16.5} & \textbf{0.2} & \underline{49.0} & 17.6 \\
Qwen2.5-Coder-7B-Ins & \textbf{84.1} &\underline{65.9} & \textbf{71.7} & \underline{64.8} & 18.4 & \underline{60.4} & 13.2 & 0.0 & 48.8 & \underline{20.3} \\
\rowcolor{lightblue}
Z1-Coder-7B & \textbf{84.1} & \textbf{69.5} & \underline{71.2} & \textbf{65.8} & \textbf{20.7} & \textbf{60.8} & \textbf{20.0} & 0.0 & \textbf{51.4} &\textbf{25.7} \\
\bottomrule
\end{tabular}
}
\end{table}

\begin{table}[h]
\centering
\small

\caption{Comparison between Z1-Coder-7B and Qwen2.5-Coder-Instruct.}
\begin{tabular}{l|c|c}
\toprule
\textbf{Model}                   & \textbf{Z1-Coder-7B} & \textbf{Qwen2.5-Coder-7B-Ins} \\
\midrule
Base Model                  & Qwen2.5-Coder-7B     & Qwen2.5-Coder-7B                  \\
SFT Data \textit{stage 1} & 110K (open-source)   & 10M+ (open-source and in-house)   \\
SFT Data \textit{stage 2}& 20K (open-source)    & 1M+ (in-house)                    \\
Offline RL      & None                   & DPO                               \\
\bottomrule
\end{tabular}
\end{table}

\begin{figure}[h]
    \centering
    \includegraphics[width=\linewidth]{fig/fig1.pdf}
    \caption{The pass@1 results of different LLMs on BigCodeBench and LiveCodeBench.}
    \label{fig1:teaser}
\end{figure}
