# Supplementary material for: Z1: Efficient Test-time Scaling with Code
Source: arXiv:2504.00810 source file (2025-04-01)
Supplement: Supplementary file 3 [file appendix-case3.tex]

% \documentclass{article}
% \usepackage[utf8]{inputenc}
% \usepackage[T1]{fontenc}
% \usepackage{xcolor}
% \usepackage{tcolorbox}
% \tcbuselibrary{listings, breakable, skins} % 加载必要的 tcolorbox 库
% \usepackage{listings}
% \usepackage{lipsum} % 用于生成示例文本

% % 设置 listings 的基本样式
% \lstset{
%     basicstyle=\tiny\ttfamily, % 字体调小为 footnotesize，并使用等宽字体
%     breaklines=true,                  % 自动换行
%     breakatwhitespace=true,           % 只在空白处换行
%     columns=flexible,                 % 灵活调整字符间距
%     breakindent=0pt,
%     mathescape=true,
% }

% \begin{document}

\begin{tcolorbox}[enhanced jigsaw, breakable,
    colback=white, colframe=black, coltitle=white,
    fonttitle=\small\bfseries,        % 标题字体保持 small
    fontupper=\scriptsize,   % 正文字体设置为 scriptsize 等宽
    rounded corners,
    title=Example SWE Manager Task 1,
    listing engine=listings,
    listing options={language=Python, breaklines=true, breakatwhitespace=true, columns=flexible}]
% \begin{lstlisting}
Consider this density matrix 
$\rho=\frac{1}{2}\left(\left|0\right\rangle \left\langle 0\right|+\left|1\right\rangle \left\langle 1\right|\right)$
What is its geometrical position in the qubits space?

A. r=(0,0,0)
B. r=(1,1,1)
C. r=(1,1,0)
D. r=(0,0,1)

Please reason step-by-step and put your choice letter without any other text with \/boxed\{\} in the end.

% \end{lstlisting}
\end{tcolorbox}
\vspace{-13pt}
% 开始并列布局
\hspace*{-1.7cm} % 向左移动左边框 0.5cm
\begin{minipage}[t]{0.6\linewidth} % 左边栏，占 48% 宽度
\begin{tcolorbox}[enhanced jigsaw, breakable,
    colback=white, colframe=blue!20, coltitle=black,
    fonttitle=\small\bfseries,        % 标题字体调小
    fontupper=\tiny,   % 正文字体设置为 scriptsize 等宽
    rounded corners,
    title=Example SWE Manager Task 1,
    listing engine=listings,
    listing options={language=Python, breaklines=true, breakatwhitespace=true, columns=flexible, mathescape=true,}]
% \begin{lstlisting}
<think>
Okay, so I have this density matrix given by 

\[\rho = (1/2)(|0⟩⟨0| + |1⟩⟨1|). \]

I need to figure out its geometrical position in the qubit space. The options are A through D, each with different coordinates. Hmm, I remember that density matrices are used in quantum mechanics to describe the state of a system, especially when it's mixed or entangled. But I'm a bit fuzzy on how to visualize this in the qubit space.

First, let me recall that a single qubit can be represented in a Bloch sphere, which is a geometrical representation of the state of a qubit. The Bloch sphere is a unit sphere in three-dimensional space, where each point corresponds to a possible state of the qubit. The pure states are represented by points on the surface of the sphere, while mixed states are inside the sphere.

The density matrix given here is 
\begin{equation}
    \rho = (|0⟩⟨0| + |1⟩⟨1|)/2
\end{equation}

Wait, that looks familiar. Isn't that the density matrix for a completely mixed state? Because when you have a completely mixed state, the density matrix is the identity matrix divided by the dimension of the space. For a qubit, which is a two-level system, the identity matrix is 2x2, so dividing by 2 gives us exactly this \rho.

But how does this correspond to a point in the qubit space? I think the completely mixed state should correspond to the center of the Bloch sphere, right? Because the center is the average of all possible pure states. So, in the Bloch sphere, the center is at (0,0,0). Let me check if that makes sense.

In the Bloch sphere representation, a pure state |ψ⟩ can be written as |ψ⟩ = cos(θ/2)|0⟩ + e^{iφ} sin(θ/2)|1⟩. The corresponding density matrix is |ψ⟩⟨ψ|. The Bloch vector for this state is (x, y, z) where x = sinθ cosφ, y = sinθ sinφ, and z = cosθ. So, for the pure states, the Bloch vector has a magnitude of 1, which places it on the surface of the sphere.

But for the mixed state, since it's a completely mixed state, it doesn't have a definite phase or any coherence. So, it's like averaging over all possible states. That should correspond to the origin, which is (0,0,0) in the Bloch sphere. So, the density matrix $\rho$ given here is the completely mixed state, which is at the center of the Bloch sphere.

Looking back at the options, A is (0,0,0), which would be the center. The other options are points on the surface or different points inside the sphere. Since the completely mixed state is at the center, the answer should be A.

Wait, let me make sure I'm not confusing anything. The density matrix for a mixed state is diagonal in the computational basis, which this one is. So, it's a classical mixture of |0⟩ and |1⟩, each with probability 1/2. In the Bloch sphere, a diagonal density matrix corresponds to a state with no coherence, meaning no y-component in the Bloch vector. So, the Bloch vector should lie along the z-axis. But since it's a completely mixed state, the z-component is zero as well. So, the Bloch vector is (0,0,0), which is the center.

Yes, that makes sense. So, the geometrical position is the origin, which is option A.

**Final Answer**
\boxed{A}
</think>

The given density matrix is 

\[
\rho = \frac{1}{2}\left(\left|0\right\rangle \left\langle 0\right| + \left|1\right\rangle \left\langle 1\right|\right)
\]

This density matrix represents a completely mixed state. In the context of a qubit, a completely mixed state corresponds to the center of the Bloch sphere. The Bloch sphere is a geometrical representation where pure states lie on the surface, and mixed states lie inside. The completely mixed state, being an average of all possible pure states, is at the origin of the Bloch sphere, which corresponds to the point (0,0,0).

Thus, the geometrical position of the given density matrix in the qubit space is the origin.

\[
\boxed{A}
\]

% \end{lstlisting}
\end{tcolorbox}
\end{minipage}%
\hfill % 添加间距
\begin{minipage}[t]{0.6\linewidth} % 右边栏，占 48% 宽度
\begin{tcolorbox}[enhanced jigsaw, breakable,
    colback=white, colframe=orange!20, coltitle=black,
    fonttitle=\small\bfseries,        % 标题字体调小
    fontupper=\tiny,   % 正文字体设置为 scriptsize 等宽
    rounded corners,
    title=Example SWE Manager Task 2,
    listing engine=listings,
    listing options={language=Python, breaklines=true, breakatwhitespace=true, columns=flexible}]
% \begin{lstlisting}
To determine the geometrical position of the given density matrix in the qubits space, we need to understand the relationship between density matrices and Bloch vectors in quantum mechanics.

First, recall that for a single qubit, the density matrix can be expressed in terms of the Bloch vector \(\mathbf{r} = (r_x, r_y, r_z)\) as:

\[
\rho = \frac{1}{2} \left( \mathbb{I} + \mathbf{r} \cdot \mathbf{\sigma} \right)
\]

where \(\mathbb{I}\) is the identity matrix and \(\mathbf{\sigma} = (\sigma_x, \sigma_y, \sigma_z)\) are the Pauli matrices.

Given the density matrix:

\[
\rho = \frac{1}{2} \left( |0\rangle \langle 0| + |1\rangle \langle 1| \right)
\]

we can see that this is a diagonal matrix with equal probabilities for the states \(|0\rangle\) and \(|1\rangle\). This corresponds to a maximally mixed state.

To find the Bloch vector \(\mathbf{r}\), we can use the expression for \(\rho\) in terms of \(\mathbf{r}\):

\[
\rho = \frac{1}{2} \left( \mathbb{I} + \mathbf{r} \cdot \mathbf{\sigma} \right)
\]

Given that \(\rho\) is:

\[
\rho = \frac{1}{2} \left( |0\rangle \langle 0| + |1\rangle \langle 1| \right) = \frac{1}{2} \begin{pmatrix} 1 & 0 \\ 0 & 1 \end{pmatrix}
\]

we can equate this to the Bloch vector expression:

\[
\frac{1}{2} \begin{pmatrix} 1 & 0 \\ 0 & 1 \end{pmatrix} = \frac{1}{2} \left( \mathbb{I} + \mathbf{r} \cdot \mathbf{\sigma} \right)
\]

This implies:

\[
\mathbb{I} = \mathbb{I} + \mathbf{r} \cdot \mathbf{\sigma}
\]

Subtracting \(\mathbb{I}\) from both sides:

\[
0 = \mathbf{r} \cdot \mathbf{\sigma}
\]

This means that the Bloch vector \(\mathbf{r}\) is orthogonal to all Pauli matrices, which is only possible if \(\mathbf{r} = (0, 0, 0)\).

Therefore, the geometrical position of the density matrix in the qubits space is at the origin.

\boxed{A}

% \end{lstlisting}
\end{tcolorbox}
\end{minipage}

% \end{document}
